# Supplementary material for: ML Based Lineage in Databases
Source: arXiv:2109.06339 source file (2021-10-03)
Supplement: Supplementary file 1 [file appendix_bfpdb_mvws.tex]

\chapter{BFPDB Materialized Views}
\label{appendix:bfpdb_materiazlied_views}

Following is a detailed description of the materialized views (used in the experiments in section \ref{sec:advanced_experiments}) and the queries that created them.

\section{\texttt{prepared}}\label{appendix:sec:prepared}
Contains all the products-related information from the \texttt{products} table, for products that have a \textit{prepared} preparation state in the \texttt{serving\_size} table:
\newcommand{\sqlcolor}[1]{\textcolor{Bittersweet}{#1}}
\newcommand{\fieldcolor}[1]{\textcolor{Fuchsia}{#1}}
\newcommand{\strcolor}[1]{\textcolor{ForestGreen}{#1}}
\newcommand{\numcolor}[1]{\textcolor{TealBlue}{#1}}

% \begin{adjustbox}{width=\columnwidth,center}
\begin{figure}[h]
% \raggedright
% \begin{small}
    \texttt{
    % \textcolor{white}{\tiny something}\\
    \textcolor{white}{F}\sqlcolor{SELECT} p.\fieldcolor{ndb\_no}, p.\fieldcolor{manufacturer}, p.\fieldcolor{name}, p.\fieldcolor{ingredients} \\
    \textcolor{white}{FF}\sqlcolor{FROM} products p, serving\_size ss\\
    \textcolor{white}{FF}\sqlcolor{WHERE} p.\fieldcolor{ndb\_no} = ss.\fieldcolor{ndb\_no} \\ 
    \textcolor{white}{FF}\sqlcolor{AND} ss.\fieldcolor{preparation\_state} = \strcolor{'prepared'}
    }
    % \textbf{\caption{\label{fig:queries_usda_bpfd}Running example query for the USDA Branded Products Food Database}}
% \end{small}
\end{figure}
% \end{adjustbox}

\section{\texttt{unprepared}}\label{appendix:sec:unprepared}
Contains all the products-related information from the \texttt{products} table, for products that have a \textit{unprepared} preparation state in the \texttt{serving\_size} table:
% \begin{adjustbox}{width=\columnwidth,center}
\begin{figure}[h]
% \raggedright
% \begin{small}
    \texttt{
    % \textcolor{white}{\tiny something}\\
    \textcolor{white}{F}\sqlcolor{SELECT} p.\fieldcolor{ndb\_no}, p.\fieldcolor{manufacturer}, p.\fieldcolor{name}, p.\fieldcolor{ingredients} \\
    \textcolor{white}{FF}\sqlcolor{FROM} products p, serving\_size ss\\
    \textcolor{white}{FF}\sqlcolor{WHERE} p.\fieldcolor{ndb\_no} = ss.\fieldcolor{ndb\_no} \\ 
    \textcolor{white}{FF}\sqlcolor{AND} ss.\fieldcolor{preparation\_state} = \strcolor{'unprepared'}
    }
    % \textbf{\caption{\label{fig:queries_usda_bpfd}Running example query for the USDA Branded Products Food Database}}
% \end{small}
\end{figure}
% \end{adjustbox}

\section{\texttt{readytodrink}}\label{appendix:sec:readytodrink}
Contains all the products-related information from the \texttt{products} table, for products that have a \textit{readytodrink} preparation state in the \texttt{serving\_size} table:
% \begin{adjustbox}{width=\columnwidth,center}
\begin{figure}[h]
% \raggedright
% \begin{small}
    \texttt{
    % \textcolor{white}{\tiny something}\\
    \textcolor{white}{F}\sqlcolor{SELECT} p.\fieldcolor{ndb\_no}, p.\fieldcolor{manufacturer}, p.\fieldcolor{name}, p.\fieldcolor{ingredients} \\
    \textcolor{white}{FF}\sqlcolor{FROM} products p, serving\_size ss\\
    \textcolor{white}{FF}\sqlcolor{WHERE} p.\fieldcolor{ndb\_no} = ss.\fieldcolor{ndb\_no} \\ 
    \textcolor{white}{FF}\sqlcolor{AND} ss.\fieldcolor{preparation\_state} = \strcolor{'readytodrink'}
    }
    % \textbf{\caption{\label{fig:queries_usda_bpfd}Running example query for the USDA Branded Products Food Database}}
% \end{small}
\end{figure}
% \end{adjustbox}

\section{\texttt{protein}}\label{appendix:sec:protein}
Contains all the products-related information from the \texttt{products} table, for products that have a \textit{protein} nutrient-related information in the \texttt{nutrients} table:
% \begin{adjustbox}{width=\columnwidth,center}
\begin{figure}[H]
% \raggedright
% \begin{small}
    \texttt{
    % \textcolor{white}{\tiny something}\\
    \textcolor{white}{F}\sqlcolor{SELECT} p.\fieldcolor{ndb\_no}, p.\fieldcolor{manufacturer}, p.\fieldcolor{name}, p.\fieldcolor{ingredients} \\
    \textcolor{white}{FF}\sqlcolor{FROM} products p, nutrients n\\
    \textcolor{white}{FF}\sqlcolor{WHERE} p.\fieldcolor{ndb\_no} = n.\fieldcolor{ndb\_no} \\ 
    \textcolor{white}{FF}\sqlcolor{AND} n.\fieldcolor{nutrient\_name} = \strcolor{'protein'}
    }
    % \textbf{\caption{\label{fig:queries_usda_bpfd}Running example query for the USDA Branded Products Food Database}}
% \end{small}
\end{figure}
% \end{adjustbox}

\section{\texttt{sugars}}\label{appendix:sec:sugars}
Contains all the products-related information from the \texttt{products} table, for products that have a \textit{sugars} nutrient-related information in the \texttt{nutrients} table:
% \begin{adjustbox}{width=\columnwidth,center}
\begin{figure}[H]
% \raggedright
% \begin{small}
    \texttt{
    % \textcolor{white}{\tiny something}\\
    \textcolor{white}{F}\sqlcolor{SELECT} p.\fieldcolor{ndb\_no}, p.\fieldcolor{manufacturer}, p.\fieldcolor{name}, p.\fieldcolor{ingredients} \\
    \textcolor{white}{FF}\sqlcolor{FROM} products p, nutrients n\\
    \textcolor{white}{FF}\sqlcolor{WHERE} p.\fieldcolor{ndb\_no} = n.\fieldcolor{ndb\_no} \\ 
    \textcolor{white}{FF}\sqlcolor{AND} n.\fieldcolor{nutrient\_name} = \strcolor{'sugars'}
    }
    % \textbf{\caption{\label{fig:queries_usda_bpfd}Running example query for the USDA Branded Products Food Database}}
% \end{small}
\end{figure}
% \end{adjustbox}

\section{\texttt{cholesterol}}\label{appendix:sec:cholesterol}
Contains all the products-related information from the \texttt{products} table, for products that have a \textit{cholesterol} nutrient-related information in the \texttt{nutrients} table:
% \begin{adjustbox}{width=\columnwidth,center}
\begin{figure}[H]
% \raggedright
% \begin{small}
    \texttt{
    % \textcolor{white}{\tiny something}\\
    \textcolor{white}{F}\sqlcolor{SELECT} p.\fieldcolor{ndb\_no}, p.\fieldcolor{manufacturer}, p.\fieldcolor{name}, p.\fieldcolor{ingredients} \\
    \textcolor{white}{FF}\sqlcolor{FROM} products p, nutrients n\\
    \textcolor{white}{FF}\sqlcolor{WHERE} p.\fieldcolor{ndb\_no} = n.\fieldcolor{ndb\_no} \\ 
    \textcolor{white}{FF}\sqlcolor{AND} n.\fieldcolor{nutrient\_name} = \strcolor{'cholesterol'}
    }
    % \textbf{\caption{\label{fig:queries_usda_bpfd}Running example query for the USDA Branded Products Food Database}}
% \end{small}
\end{figure}
% \end{adjustbox}

\section{$\texttt{exp}\sb\texttt{1}$}\label{appendix:sec:exp1}
Contains distinct manufacturers of products that have \textit{sugar} as an ingredient, and contain \textit{protein} nutrient information. Also, these manufacturers produce \textit{prepared} products: 
% \begin{adjustbox}{width=\columnwidth,center}
\begin{figure}[H]
% \raggedright
% \begin{small}
    \texttt{
    % \textcolor{white}{\tiny something}\\
    \textcolor{white}{F}\sqlcolor{SELECT} prt.\fieldcolor{manufacturer} \\
    \textcolor{white}{FF}\sqlcolor{FROM} protein prt, (\sqlcolor{SELECT DISTINCT} \fieldcolor{manufacturer} \sqlcolor{FROM} prepared) t\\
    \textcolor{white}{FF}\sqlcolor{WHERE POSITION}(\strcolor{'sugar'} \sqlcolor{IN} prt.\fieldcolor{ingredients}) > \numcolor{0} \\
    \textcolor{white}{FF}\sqlcolor{AND} prt.\fieldcolor{manufacturer} = t.\fieldcolor{manufacturer}\\
    \textcolor{white}{FF}\sqlcolor{GROUP BY} prt.\fieldcolor{manufacturer}
    }
    % \textbf{\caption{\label{fig:queries_usda_bpfd}Running example query for the USDA Branded Products Food Database}}
% \end{small}
\end{figure}
% \end{adjustbox}

\section{$\texttt{exp}\sb\texttt{2}$}\label{appendix:sec:exp2}
Contains distinct manufacturers of products that have \textit{water} as an ingredient, and contain \textit{protein} nutrient information. Also, these manufacturers produce \textit{unprepared} products: 
% \begin{adjustbox}{width=\columnwidth,center}
\begin{figure}[H]
% \raggedright
% \begin{small}
    \texttt{
    % \textcolor{white}{\tiny something}\\
    \textcolor{white}{F}\sqlcolor{SELECT} prt.\fieldcolor{manufacturer} \\
    \textcolor{white}{FF}\sqlcolor{FROM} protein prt, (\sqlcolor{SELECT DISTINCT} \fieldcolor{manufacturer} \sqlcolor{FROM} unprepared) t\\
    \textcolor{white}{FF}\sqlcolor{WHERE POSITION}(\strcolor{'water'} \sqlcolor{IN} prt.\fieldcolor{ingredients}) > \numcolor{0} \\
    \textcolor{white}{FF}\sqlcolor{AND} prt.\fieldcolor{manufacturer} = t.\fieldcolor{manufacturer}\\
    \textcolor{white}{FF}\sqlcolor{GROUP BY} prt.\fieldcolor{manufacturer}
    }
    % \textbf{\caption{\label{fig:queries_usda_bpfd}Running example query for the USDA Branded Products Food Database}}
% \end{small}
\end{figure}
% \end{adjustbox}

\section{$\texttt{exp}\sb\texttt{3}$}\label{appendix:sec:exp3}
Contains distinct manufacturers of products that have \textit{water} and \textit{sugar} as an ingredient, and contain \textit{protein} nutrient information. Also, these manufacturers produce \textit{prepared} and \textit{unprepared} products:
% \begin{adjustbox}{width=\columnwidth,center}
\begin{figure}[H]
% \raggedright
% \begin{small}
    \texttt{
    % \textcolor{white}{\tiny something}\\
    \textcolor{white}{F}\sqlcolor{SELECT} $\texttt{t}\sb\texttt{2}$.\fieldcolor{manufacturer} \sqlcolor{FROM}\\
    \textcolor{white}{FFFF}(\sqlcolor{SELECT} prt.\fieldcolor{manufacturer} \\
    \textcolor{white}{FFFFF}\sqlcolor{FROM} protein prt, (\sqlcolor{SELECT DISTINCT} \fieldcolor{manufacturer} \sqlcolor{FROM} prepared) t\\
    \textcolor{white}{FFFFF}\sqlcolor{WHERE POSITION}(\strcolor{'sugar'} \sqlcolor{IN} prt.\fieldcolor{ingredients}) > \numcolor{0} \\
    \textcolor{white}{FFFFF}\sqlcolor{AND} prt.\fieldcolor{manufacturer} = t.\fieldcolor{manufacturer}\\
    \textcolor{white}{FFFFF}\sqlcolor{GROUP BY} prt.\fieldcolor{manufacturer}) $\texttt{t}\sb\texttt{1}$,\\
    \textcolor{white}{FFFF}(\sqlcolor{SELECT} prt.\fieldcolor{manufacturer} \\
    \textcolor{white}{FFFFF}\sqlcolor{FROM} protein prt, (\sqlcolor{SELECT DISTINCT} \fieldcolor{manufacturer} \sqlcolor{FROM} unprepared) t\\
    \textcolor{white}{FFFFF}\sqlcolor{WHERE POSITION}(\strcolor{'water'} \sqlcolor{IN} prt.\fieldcolor{ingredients}) > \numcolor{0} \\
    \textcolor{white}{FFFFF}\sqlcolor{AND} prt.\fieldcolor{manufacturer} = t.\fieldcolor{manufacturer}\\
    \textcolor{white}{FFFFF}\sqlcolor{GROUP BY} prt.\fieldcolor{manufacturer}) $\texttt{t}\sb\texttt{2}$,\\
    \textcolor{white}{FF}\sqlcolor{WHERE} $\texttt{t}\sb\texttt{1}$.\fieldcolor{manufacturer} = $\texttt{t}\sb\texttt{2}$.\fieldcolor{manufacturer}
    }
    % \textbf{\caption{\label{fig:queries_usda_bpfd}Running example query for the USDA Branded Products Food Database}}
% \end{small}
\end{figure}
% \end{adjustbox}

\section{$\texttt{exp}\sb\texttt{4}$}\label{appendix:sec:exp4}
Contains distinct names of products from the \texttt{readytodrink} materialized view, that contain \textit{mango} in their name, and are produced by manufacturers from the $\texttt{exp}\sb\texttt{2}$ materialized view:
% \begin{adjustbox}{width=\columnwidth,center}
\begin{figure}[H]
% \raggedright
% \begin{small}
    \texttt{
    % \textcolor{white}{\tiny something}\\
    \textcolor{white}{F}\sqlcolor{SELECT DISTINCT} rtd.\fieldcolor{name} \\
    \textcolor{white}{FF}\sqlcolor{FROM} $\texttt{exp}\sb\texttt{2}$, readytodrink rtd\\
    \textcolor{white}{FF}\sqlcolor{WHERE} $\texttt{exp}\sb\texttt{2}$.\fieldcolor{manufacturer} = rtd.\fieldcolor{manufacturer}\\
    \textcolor{white}{FF}\sqlcolor{AND POSITION}(\strcolor{'mango'} \sqlcolor{IN} rtd.\fieldcolor{name}) > \numcolor{0}
    }
    % \textbf{\caption{\label{fig:queries_usda_bpfd}Running example query for the USDA Branded Products Food Database}}
% \end{small}
\end{figure}
% \end{adjustbox}
