# Supplementary material for: ML Based Lineage in Databases
Source: arXiv:2109.06339 source file (2021-10-03)
Supplement: Supplementary file 2 [file appendix_bfpdb_schema.tex]

\chapter{BFPDB Dataset}
\label{appendix:bfpdb_schema}

Following is a detailed description of the data fields, of each table in the BFPDB dataset (used in the experiments in chapter \ref{chap:experimental_evaluation}).

\section{\texttt{products}}\label{appendix:sec:products}
\begin{itemize}
    \item \textbf{\texttt{ndb\_no}} - 8-digit Nutrient Database (NDB) number that uniquely identifies a food item. Links to the \texttt{nutrients} table and the \texttt{serving\_size} table.
    \item \textbf{\texttt{name}} - 200-character description of a food item.
    \item \textbf{\texttt{manufacturer}} - the company that manufactured the product.
    \item \textbf{\texttt{ingredients}} - ingredients of the product.
\end{itemize}

\section{\texttt{nutrients}}\label{appendix:sec:nutrients}
% \subsection{Fields Description}
\begin{itemize}
    \item \textbf{\texttt{ndb\_no}} - 8-digit Nutrient Database (NDB) number that uniquely identifies a food item. Links to the \texttt{products} table and the \texttt{serving\_size} table.
    \item \textbf{\texttt{nutrient\_code}} - unique 3-digit identifier code for a nutrient.
    \item \textbf{\texttt{nutrient\_name}} - name of nutrient/food component.
    \item \textbf{\texttt{derivation\_code}} - a code indicating how the \texttt{output\_value} was determined. The codes used are defined in the \texttt{derivation\_code\_description} table.
    \item \textbf{\texttt{output\_value}} - amount in 100 g, edible portion. This value is calculated from the amount per serving value on the Nutrition Facts Panel supplied by the data provider.
    \item \textbf{\texttt{output\_uom}} - units of measure for the \texttt{output\_value}.
\end{itemize}
% \subsection{Sample}
% \input{tables/bfpdb_samples/nutrients}

\section{\texttt{serving\_size}}\label{appendix:sec:serving-size}
\begin{itemize}
    \item \textbf{\texttt{ndb\_no}} - 8-digit Nutrient Database (NDB) number that uniquely identifies a food item. Links to the \texttt{products} table and the \texttt{nutrients} table.
    \item \textbf{\texttt{household\_serving}} - the amount of the \texttt{household\_serving\_size\_uom}, i.e., the number of cups, tablespoons, teaspoons in a serving. May be a fraction, such as 0.25 or 0.50.
    \item \textbf{\texttt{household\_serving\_size\_uom}} - the Units of Measure for the \texttt{household\_serving}, i.e., cup, tablespoon, teaspoon.
    \item \textbf{\texttt{preparation\_state}} - indicates if the information from the Nutrition Facts Panel is for the prepared or unprepared food. Only included if supplied.
\end{itemize}

\section{\texttt{derivation\_code\_description}}\label{appendix:sec:dcd}
\begin{itemize}
    \item \textbf{\texttt{derivation\_code}} - a code indicating how the \texttt{output\_value} was determined. Links to the \texttt{nutrients} table.
    \item \textbf{\texttt{derivation\_code\_description}} - description of the \texttt{derivation\_code}.
\end{itemize}
