# Supplementary material for: ML Based Lineage in Databases
Source: arXiv:2109.06339 source file (2021-10-03)
Supplement: Supplementary file 3 [file appendix_efficient_vector_search.tex]

\chapter{Efficient Set of Vectors Search}
\label{appendix:efficient_vectors_search}

\section{Rationale}
In this work, we obtain a lineage via an embedding based method, such that each tuple/column (see chapters \ref{chap:per_tuple_lineage_vectors} and \ref{chap:per_column_lineage_vectors}) is associated with a \textit{set of vectors}.
We want to adapt known approximate vector search algorithms (e.g., based on LSH \cite{lsh}) to efficiently implement our method (we define a ``similarity between two sets of vectors" formula in section \ref{sec:similarity_calculation}). That is, we need an efficient approximate search algorithm of nearest sets of lineage vectors. We then can utilize this algorithm in lineage querying for locating contributors, instead of comparing a target tuple explicitly with all of its lineage candidates and sorting them by similarity.
\par First, we present a basic method under the assumption that all the sets of lineage vectors in the DB are of a constant cardinality $N$. Then, we introduce a refined version that supports sets of vectors of varying cardinalities, such that each set of vectors $V$, which is associated with a tuple or a tuple column in the DB, has a cardinality $|V| \in [1, max\_vectors\_num]$ ($max\_vectors\_num$ is a hyperparameter of our system).

\section{A Constant Cardinality of Sets of Vectors}
Here, we assume that all the sets of lineage vectors in the DB are of a constant cardinality $N$. The idea is transforming each set of vectors into a single long vector, so that the \textit{dot product} of two such long vectors computes all pair-wise interactions, and is equivalent to the similarity calculation (between sets of vectors) we devised in section \ref{sec:similarity_calculation}. Note that all the lineage vectors in the DB have the same constant dimension $D$ (a hyperparameter of our system).

\subsection{Implementation}\label{sec:constant_cardinality_vector_search}
% Suppose a lineage target tuple $t_A$ is associated with a set $A$ of lineage vectors.

\subsubsection{Long Vectors Construction}
\begin{enumerate}
    \item Suppose a target tuple $t_A$ is associated with a set $A$ of lineage vectors of cardinality $N$.
    % \item Let $t_V$ be a lineage candidate tuple for $t_A$, that is associated with a set $V$ of lineage vectors. 
    % \item Let $A$ and $V$ be two sets of lineage vectors. Suppose w.l.o.g. that $A$ is associated with a lineage target tuple $t_A$ and $V$ is associated with a lineage candidate tuple $t_V$.
    \item Let $t_V$ be a candidate tuple for $t_A$, that is associated with a set $V$ of lineage vectors of cardinality $N$. Construct a \textit{long candidate vector} $\vec{L}_V \in \mathbb{R}^{|A| \times |V| \times D}$ from $V$ by concatenating $|A|$ copies of each (normalized) $\vec{v}_i \in V$, in order $\vec{v}_1, ..., \vec{v}_{|V|}$: \\
    \begin{equation*}
        \vec{L}_V = \begin{pmatrix}
                    \frac{\vec{v}_{1, 1}}{\lVert \vec{v}_1 \rVert}\\ 
                    \vdots\\ 
                    \frac{\vec{v}_{1, |A|}}{\lVert \vec{v}_1 \rVert}\\ 
                   \vdots\\ 
                   \frac{\vec{v}_{|V|, 1}}{\lVert \vec{v}_{|V|} \rVert}\\ 
                   \vdots\\ 
                   \frac{\vec{v}_{|V|, |A|}}{\lVert \vec{v}_{|V|} \rVert}\\
                   \end{pmatrix}
                  \underset{\scriptscriptstyle |A| = |V| = N}{=} 
                  \begin{pmatrix}
                    \frac{\vec{v}_{1, 1}}{\lVert \vec{v}_1 \rVert}\\ 
                    \vdots\\ 
                    \frac{\vec{v}_{1, N}}{\lVert \vec{v}_1 \rVert}\\ 
                   \vdots\\ 
                   \frac{\vec{v}_{N, 1}}{\lVert \vec{v}_N \rVert}\\ 
                   \vdots\\ 
                   \frac{\vec{v}_{N, N}}{\lVert \vec{v}_N \rVert}\\
                   \end{pmatrix}
                   \end{equation*}
        such that $\vec{v}_{i, j}$ is the $j^{th}$ copy of $\vec{v}_i$.
    \item Now, we build a long vector $\vec{L}_{A} \in \mathbb{R}^{|A| \times |V| \times D}$ by concatenating all (normalized) $\vec{a}_i \in A$, in order $\vec{a}_1, ..., \vec{a}_{|A|}$, and duplicating the result $|V|$ times: \\
    \begin{equation*}
        \vec{L}_{A} = \begin{pmatrix}
                    \frac{\vec{a}_{1, 1}}{\lVert \vec{a}_1 \rVert}\\ 
                    \vdots\\ 
                    \frac{\vec{a}_{|A|, 1}}{\lVert \vec{a}_{|A|} \rVert}\\ 
                   \vdots\\ 
                   \frac{\vec{a}_{1, |V|}}{\lVert \vec{a}_{1} \rVert}\\ 
                   \vdots\\ 
                   \frac{\vec{a}_{|A|, |V|}}{\lVert \vec{a}_{|A|} \rVert}\\
                   \end{pmatrix}
                  \underset{\scriptscriptstyle |A| = |V| = N}{=} 
                  \begin{pmatrix}
                     \frac{\vec{a}_{1, 1}}{\lVert \vec{a}_1 \rVert}\\ 
                    \vdots\\ 
                    \frac{\vec{a}_{N, 1}}{\lVert \vec{a}_{N} \rVert}\\ 
                   \vdots\\ 
                   \frac{\vec{a}_{1, N}}{\lVert \vec{a}_{1} \rVert}\\ 
                   \vdots\\ 
                   \frac{\vec{a}_{N, N}}{\lVert \vec{a}_{N} \rVert}\\
                   \end{pmatrix}
                   \end{equation*}
       such that $\vec{a}_{i, j}$ is the $j^{th}$ copy of $\vec{a}_i$.
    \item $\vec{L}_{A}$ is used to capture the \textit{average} of all pair-wise \textit{cosine similarities} with vectors from a candidate set $V$ (note that $a_{i, j} = a_i$ and $v_{j, i} = v_j$):\\
    \begin{equation*}
        \vec{L}_{A} \cdot \vec{L}_V = \sum_{i = 1}^{|A|}{\sum_{j = 1}^{|V|} \frac{\vec{a}_{i, j}}{\lVert \vec{a}_i \rVert} \cdot \frac{\vec{v}_{j, i}}{\lVert \vec{v}_j \rVert}} = sum(ps) = avg(ps) \times |A| \times |V| \underset{\scriptscriptstyle |A| = |V| = N}{=} avg(ps) \times N^2
    \end{equation*}
    where $ps$ is the multi-set of pair-wise similarities between a pair of vectors, one taken from set $V$ and one taken from set $A$.
    \item To capture the maximum of the pair-wise similarities (denoted $max(ps)$) we build $|A| \times |V| = N^2$ long ``selector" vectors $\vec{\sigma}_{1, 1}, ..., \vec{\sigma}_{|A|, 1}, ..., \vec{\sigma}_{1, |V|}, ..., \vec{\sigma}_{|A|, |V|}$, each $\vec{\sigma}_{i, j} \in \mathbb{R}^{|A| \times |V| \times D}$ ``assumes" which of the $|A| \times |V| = N^2$ pair-wise interactions is maximal:\\
    \begin{equation*}
        \vec{\sigma}_{i, j} = \begin{pmatrix}
                    \vec{0}_{1, 1}\\ 
                    \vdots\\ 
                    \vec{0}_{|A|, 1}\\ 
                   \vdots\\
                   \vec{1}_{i, j}\\ 
                   \vdots\\
                   \vec{0}_{1, |V|}\\ 
                   \vdots\\ 
                   \vec{0}_{|A|, |V|}\\ 
                   \end{pmatrix}
    \end{equation*}
    i.e., $\vec{\sigma}_{i, j}$ is a concatenation of $O_s = (j - 1) \times |A| + (i - 1)$ $\vec{0}$ vectors, followed by one $\vec{1}$ vector, and ending with $|A| \times |V| - (O_s + 1)$ $\vec{0}$ vectors,
    where $\vec{0} \in \mathbb{R}^D$ is the ``all zeros" vector and $\vec{1} \in \mathbb{R}^D$ is the ``all ones" vector. 
    $\vec{\sigma}_{i, j}$ ``assumes" the maximum occurs in the cosine similarity product between $\vec{a}_i$ and $\vec{v}_j$.
    Consequently, we get:\\
    \begin{equation*}
        \vec{\sigma}_{i, j} \odot \vec{L}_{A} = \begin{pmatrix}
                    \vec{0}_{1, 1}\\ 
                    \vdots\\ 
                    \vec{0}_{|A|, 1}\\ 
                   \vdots\\
                   \frac{\vec{a}_{i, j}}{\lVert \vec{a}_i \rVert}\\ 
                   \vdots\\
                   \vec{0}_{1, |V|}\\ 
                   \vdots\\ 
                   \vec{0}_{|A|, |V|}\\ 
                   \end{pmatrix}
    \end{equation*}
    such that $\vec{a}_{i, j}$ is the $j^{th}$ copy of $\vec{a}_i$ and $\odot$ is the Hadamard (i.e., element-wise) product.
    This results in:
    \begin{equation*}
        (\vec{\sigma}_{i, j} \odot \vec{L}_{A}) \cdot \vec{L}_V = \frac{\vec{a}_{i, j}}{\lVert \vec{a}_i \rVert} \cdot \frac{\vec{v}_{j, i}}{\lVert \vec{v}_j \rVert} = \frac{\vec{a}_{i}}{\lVert \vec{a}_i \rVert} \cdot \frac{\vec{v}_{j}}{\lVert \vec{v}_j \rVert}
    \end{equation*}
    
    \item Next, we construct $|A| \times |V| = N^2$ \textit{long target vectors} $\vec{\tau}_{1, 1}, ..., \vec{\tau}_{|A|, 1}, ..., \vec{\tau}_{1, |V|}, ..., \vec{\tau}_{|A|, |V|}$ ($\vec{\tau}_{i, j} \in \mathbb{R}^{|A| \times |V| \times D}$):
    \begin{equation*}
        \vec{\tau}_{i, j} =
        \frac{1}{w_{max} + w_{avg}} \cdot \left (
        w_{max} \cdot (\vec{\sigma}_{i, j} \odot \vec{L}_{A}) 
        + \frac{w_{avg}}{|A| \times |V|} \cdot \vec{L}_{A}
        \right )
    \end{equation*}
    where $w_{max}$ and $w_{avg}$ are (user-specified) hyperparameters, as specified in section \ref{sec:similarity_calculation}.
    \item Each long target vector $\vec{\tau}_{i, j}$ computes the desired similarity calculation via a dot product with a long candidate vector $\vec{L}_V$, under the assumption that $\vec{a}_i$ and $\vec{v}_j$ have the maximal pair-wise similarity:
    \begin{equation*}
         \vec{\tau}_{i, j} \cdot \vec{L}_V = \frac{w_{max} \cdot (\vec{\sigma}_{i, j} \odot \vec{L}_{A}) \cdot \vec{L}_V + \frac{w_{avg}}{|A| \times |V|} \cdot \vec{L}_{A} \cdot \vec{L}_V}{w_{max} + w_{avg}} 
        = 
        % \frac{w_{max} \cdot \frac{\vec{v}_{i, j}}{\lVert \vec{v}_i \rVert} \cdot \frac{\vec{a}_{j, i}}{\lVert \vec{a}_j \rVert} + w_{avg} \cdot avg(ps)}{w_{max} + w_{avg}}
    \end{equation*}
    \begin{equation*}
        = 
        \frac{w_{max} \cdot \frac{\vec{a}_{i, j}}{\lVert \vec{a}_i \rVert} \cdot \frac{\vec{v}_{j, i}}{\lVert \vec{v}_j \rVert} + w_{avg} \cdot avg(ps)}{w_{max} + w_{avg}}
        = 
        \frac{w_{max} \cdot \frac{\vec{a}_{i}}{\lVert \vec{a}_i \rVert} \cdot \frac{\vec{v}_{j}}{\lVert \vec{v}_j \rVert} + w_{avg} \cdot avg(ps)}{w_{max} + w_{avg}}
    \end{equation*}
\end{enumerate}

\subsubsection{Search}
\begin{enumerate}
    \item Insert all the long \textit{candidate} vectors (of a constant dimension $N^2 \times D$), associated with tuples or tuple columns in the DB, into a vector search structure $S$. Note that known approximate vector search techniques, such as LSH \cite{lsh}, can be utilized here for efficiency.
    \item Recall that for a tuple $t_V$ (or a column of a tuple $t_V$), that is associated with a set of vectors $V$, the long candidate vector is $\vec{L}_V$.
    \item Now, suppose you are given a target tuple $t_A$, that is associated with a set $A$ of lineage vectors of cardinality $N$. Construct $N^2$ long target vectors $\vec{\tau}_{1, 1}, ..., \vec{\tau}_{N, N}$. 
    \item We look \textit{separately} for the closest (dot-product wise) long candidate vector $\vec{L}_{{i, j}}$ (and its respective candidate tuple $t_{{i, j}}$) in $S$, to each $\vec{\tau}_{i, j}$, respectively.
    \item We compute the similarity scores $\vec{\tau}_{1, 1} \cdot \vec{L}_{{1, 1}}, ..., \vec{\tau}_{N, 1} \cdot \vec{L}_{{N, 1}}, ..., \vec{\tau}_{1, N} \cdot \vec{L}_{{1, N}}, ..., \vec{\tau}_{N, N} \cdot \vec{L}_{{N, N}}$. The one yielding the highest score, say $\vec{L}_{{{\Tilde{i}, {\Tilde{j}}}}}$, identifies the desired candidate tuple $t_{{{\Tilde{i}, {\Tilde{j}}}}}$, which is associated with a set $V_{{\Tilde{i}, {\Tilde{j}}}}$ of lineage vectors, according to our set-oriented similarity formula.
\end{enumerate}

\section{Varying Cardinalities of Sets of Vectors}\label{sec:varying_cardinalities_vector_search}
In section \ref{sec:constant_cardinality_vector_search}, we presented the construction of a long candidate vector $\vec{L}_V$ from a set of lineage vectors $V$, that is associated with a candidate tuple $t_V$, and a collection of long target vectors $\vec{\tau}_{i, j}$ (where $i \in [1, |A|=N]$ and $j \in [1, |V| = N]$|) from a set of lineage vectors $A$, that is associated with a target tuple $t_A$, under the assumption that all the sets of lineage vectors in the DB are of a constant cardinality $N$. It is evident that these constructions are tightly coupled with the cardinalities of the sets of lineage vectors of the target and candidate tuples, namely $|A|$ and $|V|$.
Hence, we introduce a refined version that supports sets of vectors of varying cardinalities, such that each set of vectors 
$V$, which is associated with a tuple or a tuple column in the DB, has a cardinality $|V| \in [1, max\_vectors\_num]$ ($max\_vectors\_num$ is hereafter denoted as $M$, for brevity). 
Recall that all the lineage vectors in the DB have the same constant dimension $D$.
\par The general idea is pre-computing $M$ long candidate vectors $\vec{L}_V^1, ..., \vec{L}_V^M$ instead of a single $\vec{L}_V$, and a collection of long target vectors $\vec{\tau}_{i, j}^k$, for each $k \in [1, M]$ (where $i \in [1, |A|]$ and $j \in [1, k]$|). Each $\vec{L}_V^n \in \mathbb{R}^{n \times |V| \times D}$, where $n \in [1, M]$, ``assumes" in its construction that the cardinality of the set of lineage vectors of a target tuple is $n$. Each $\vec{\tau}_{i, j}^k \in \mathbb{R}^{|A| \times k \times D}$, where $k \in [1, M]$, ``assumes" in its construction that the cardinality of the set of lineage vectors of a candidate tuple is $k$. Consequently, instead of a \textit{single} form of long candidate and target vectors (of dimension $N^2 \times D$, as is the case in section \ref{sec:constant_cardinality_vector_search}), we potentially get $M \times M$ different such forms (in terms of dimension and $(n, k)$ construction parameters), such that each long vector of dimension $n \times k \times D$, where $n,k \in [1, M]$, is associated with a separate search structure $S_{1,1}, ..., S_{M,M}$, depending on its $(n, k)$ form (there are additional options, e.g., combining such search structures of equal dimensions).

\subsection{Implementation}

\subsubsection{Long Vectors Construction}
\begin{enumerate}

    \item Let $t_V$ be a candidate tuple, that is associated with a set $V$ of lineage vectors of cardinality $|V| \in [1, M]$. Construct $M$ long candidate vectors $\vec{L}_V^1, ..., \vec{L}_V^M$, such that each $\vec{L}_V^n \in \mathbb{R}^{n \times |V| \times D}$, where $n \in [1, M]$, is constructed from $V$ by concatenating $n$ copies of each (normalized) $\vec{v}_i \in V$, in order $\vec{v}_1, ..., \vec{v}_{|V|}$: \\
    \begin{equation*}
        \vec{L}_V^n = \begin{pmatrix}
                    \frac{\vec{v}_{1, 1}}{\lVert \vec{v}_1 \rVert}\\ 
                    \vdots\\ 
                    \frac{\vec{v}_{1, n}}{\lVert \vec{v}_1 \rVert}\\ 
                   \vdots\\ 
                   \frac{\vec{v}_{|V|, 1}}{\lVert \vec{v}_{|V|} \rVert}\\ 
                   \vdots\\ 
                   \frac{\vec{v}_{|V|, n}}{\lVert \vec{v}_{|V|} \rVert}\\
                   \end{pmatrix}
                   \end{equation*}
        such that $\vec{v}_{i, j}$ is the $j^{th}$ copy of $\vec{v}_i$.
        $\vec{L}_V^n$ ``assumes" the cardinality of the set of lineage vectors of the target tuple is $n$.
        
    \item Suppose a target tuple $t_A$ is associated with a set $A$ of lineage vectors of cardinality $|A| \in [1, M]$.

    \item Now, we build $M$ long vectors $\vec{L}_{A}^1, ..., \vec{L}_{A}^M$, such that $\vec{L}_{A}^k \in \mathbb{R}^{|A| \times k \times D}$, where $k \in [1, M]$, is built by concatenating all (normalized) $\vec{a}_i \in A$, in order $\vec{a}_1, ..., \vec{a}_{|A|}$, and duplicating the result $k$ times: \\
        \begin{equation*}
            \vec{L}_{A}^k = \begin{pmatrix}
                    \frac{\vec{a}_{1, 1}}{\lVert \vec{a}_1 \rVert}\\ 
                    \vdots\\ 
                    \frac{\vec{a}_{|A|, 1}}{\lVert \vec{a}_{|A|} \rVert}\\ 
                   \vdots\\ 
                   \frac{\vec{a}_{1, k}}{\lVert \vec{a}_{1} \rVert}\\ 
                   \vdots\\ 
                   \frac{\vec{a}_{|A|, k}}{\lVert \vec{a}_{|A|} \rVert}\\
                   \end{pmatrix}
       \end{equation*}
       such that $\vec{a}_{i, j}$ is the $j^{th}$ copy of $\vec{a}_i$.
       $\vec{L}_{A}^k$ ``assumes" the cardinality of the set of lineage vectors of the candidate tuple is $k$.
    \item Let $t_V$ be a candidate tuple for $t_A$, that is associated with a set $V$ of lineage vectors of cardinality $|V| \in [1, M]$.
   Long vector $\vec{L}_{A}^{k=|V|} \in \mathbb{R}^{|A| \times |V| \times D}$ is used to capture the \textit{average} of all pair-wise \textit{cosine similarities} with vectors from $V$ ($\vec{L}_V^{n=|A|} \in \mathbb{R}^{|A| \times |V| \times D}$):\\
    \begin{equation*}
        \vec{L}_{A}^{k=|V|} \cdot \vec{L}_V^{n=|A|} =
        \vec{L}_{A}^{|V|} \cdot \vec{L}_V^{|A|} = \sum_{i = 1}^{|A|}{\sum_{j = 1}^{|V|} \frac{\vec{a}_{i, j}}{\lVert \vec{a}_i \rVert} \cdot \frac{\vec{v}_{j, i}}{\lVert \vec{v}_j \rVert}} = sum(ps) = avg(ps) \times |A| \times |V|
    \end{equation*}
    where $ps$ is the multi-set of pair-wise similarities between a pair of vectors, one taken from set $V$ and one taken from set $A$.
    
    \item To capture the maximum of the pair-wise similarities (denoted $max(ps)$) we build $|A| \times k$ long ``selector" vectors $\vec{\sigma}_{1, 1}^k, ..., \vec{\sigma}_{|A|, 1}^k, ..., \vec{\sigma}_{1, k}^k, ..., \vec{\sigma}_{|A|, k}^k$, for each $k \in [1, M]$. 
    That is, a total of $\sum_{k=1}^M |A| \times k = |A| \times \sum_{k=1}^M k = |A| \times \frac{M(1 + M)}{2}$ long ``selector" vectors.
    Each $\vec{\sigma}_{i, j}^k \in \mathbb{R}^{|A| \times k \times D}$ ``assumes" which of the $|A| \times k$ pair-wise interactions is maximal:\\
    \begin{equation*}
        \vec{\sigma}_{i, j}^k = \begin{pmatrix}
                    \vec{0}_{1, 1}\\ 
                    \vdots\\ 
                    \vec{0}_{|A|, 1}\\ 
                   \vdots\\
                   \vec{1}_{i, j}\\ 
                   \vdots\\
                   \vec{0}_{1, k}\\ 
                   \vdots\\ 
                   \vec{0}_{|A|, k}\\ 
                   \end{pmatrix}
    \end{equation*}
    i.e., $\vec{\sigma}_{i, j}^k$ is a concatenation of $O_s = (j - 1) \times |A| + (i - 1)$ $\vec{0}$ vectors, followed by one $\vec{1}$ vector, and ending with $|A| \times k - (O_s + 1)$ $\vec{0}$ vectors,
    where $\vec{0} \in \mathbb{R}^D$ is the ``all zeros" vector and $\vec{1} \in \mathbb{R}^D$ is the ``all ones" vector. 
    $\vec{\sigma}_{i, j}^k$ ``assumes" the maximum occurs in the cosine similarity product between $\vec{a}_i$ and $\vec{v}_j$. Also, $\vec{\sigma}_{i, j}^k$ ``assumes" the cardinality of the set of lineage vectors of the candidate tuple is $k$.
    Consequently, we get:\\
    \begin{equation*}
        \vec{\sigma}_{i, j}^k \odot \vec{L}_{A}^k = \begin{pmatrix}
                    \vec{0}_{1, 1}\\ 
                    \vdots\\ 
                    \vec{0}_{|A|, 1}\\ 
                   \vdots\\
                   \frac{\vec{a}_{i, j}}{\lVert \vec{a}_i \rVert}\\ 
                   \vdots\\
                   \vec{0}_{1, k}\\ 
                   \vdots\\ 
                   \vec{0}_{|A|, k}\\ 
                   \end{pmatrix}
    \end{equation*}
    such that $\vec{a}_{i, j}$ is the $j^{th}$ copy of $\vec{a}_i$ and $\odot$ is the Hadamard (i.e., element-wise) product.
    This results in:
    \begin{equation*}
        (\vec{\sigma}_{i, j}^{k=|V|} \odot \vec{L}_{A}^{k=|V|}) \cdot \vec{L}_V^{n=|A|} =
        (\vec{\sigma}_{i, j}^{|V|} \odot \vec{L}_{A}^{|V|}) \cdot \vec{L}_V^{|A|} = \frac{\vec{a}_{i, j}}{\lVert \vec{a}_i \rVert} \cdot \frac{\vec{v}_{j, i}}{\lVert \vec{v}_j \rVert} = \frac{\vec{a}_{i}}{\lVert \vec{a}_i \rVert} \cdot \frac{\vec{v}_{j}}{\lVert \vec{v}_j \rVert}
    \end{equation*}
    
    \item Next, we construct $|A| \times k$ long target vectors $\vec{\tau}_{1, 1}^k, ..., \vec{\tau}_{|A|, 1}^k, ..., \vec{\tau}_{1, k}^k, ..., \vec{\tau}_{|A|, k}^k$ for each $k \in [1, M]$. That is, a total of $\sum_{k=1}^M |A| \times k = |A| \times \sum_{k=1}^M k = |A| \times \frac{M(1 + M)}{2}$ long target vectors $\vec{\tau}_{i, j}^k \in \mathbb{R}^{|A| \times k \times D}$:
    \begin{equation*}
        \vec{\tau}_{i, j}^k =
        \frac{1}{w_{max} + w_{avg}} \cdot \left (
        w_{max} \cdot (\vec{\sigma}_{i, j}^k \odot \vec{L}_{A}^k) 
        + \frac{w_{avg}}{|A| \times k} \cdot \vec{L}_{A}^k
        \right )
    \end{equation*}
    where $w_{max}$ and $w_{avg}$ are (user-specified) hyperparameters, as specified in section \ref{sec:similarity_calculation}. 
    $\vec{\tau}_{i, j}^k$ ``assumes" the cardinality of the set of lineage vectors of the candidate tuple is $k$.
    
    \item Each long target vector $\vec{\tau}_{i, j}^{k=|V|} \in \mathbb{R}^{|A| \times |V| \times D}$ computes the desired similarity calculation via a dot product with a long candidate vector $\vec{L}_V^{n=|A|} \in \mathbb{R}^{|A| \times |V| \times D}$, under the assumption that $\vec{a}_i$ and $\vec{v}_j$ have the maximal pair-wise similarity:
    \begin{equation*}
        \vec{\tau}_{i, j}^{k=|V|} \cdot \vec{L}_V^{n=|A|} =
         \vec{\tau}_{i, j}^{|V|} \cdot \vec{L}_V^{|A|} = \frac{w_{max} \cdot (\vec{\sigma}_{i, j}^{|V|} \odot \vec{L}_{A}^{|V|}) \cdot \vec{L}_V^{|A|} + \frac{w_{avg}}{|A| \times |V|} \cdot \vec{L}_{A}^{|V|} \cdot \vec{L}_V^{|A|}}{w_{max} + w_{avg}} 
        = 
        % \frac{w_{max} \cdot \frac{\vec{v}_{i, j}}{\lVert \vec{v}_i \rVert} \cdot \frac{\vec{a}_{j, i}}{\lVert \vec{a}_j \rVert} + w_{avg} \cdot avg(ps)}{w_{max} + w_{avg}}
    \end{equation*}
    \begin{equation*}
        = 
        \frac{w_{max} \cdot \frac{\vec{a}_{i, j}}{\lVert \vec{a}_i \rVert} \cdot \frac{\vec{v}_{j, i}}{\lVert \vec{v}_j \rVert} + w_{avg} \cdot avg(ps)}{w_{max} + w_{avg}}
        = 
        \frac{w_{max} \cdot \frac{\vec{a}_{i}}{\lVert \vec{a}_i \rVert} \cdot \frac{\vec{v}_{j}}{\lVert \vec{v}_j \rVert} + w_{avg} \cdot avg(ps)}{w_{max} + w_{avg}}
    \end{equation*}

\end{enumerate}

\subsubsection{Search}
\begin{enumerate}
    \item Initialize $M \times M$ vector search structures $S_{1,1}, ..., S_{M,M}$, such that $S_{n, k}$ holds long \textit{candidate} vectors of dimension $n \times k \times D$ (i.e., long vectors of candidate sets of cardinality $k$, assuming target sets of cardinality $n$). Note that known approximate vector search techniques, such as LSH \cite{lsh}, can be utilized here for efficiency.
    \item For each candidate tuple $t_V$, that is associated with a set $V$ of lineage vectors of cardinality $|V| \in [1, M]$, and its respective construction of $M$ long \textit{candidate} vectors $\vec{L}_V^n \in \mathbb{R}^{n \times |V| \times D}$, for each $n \in [1, M]$, insert $\vec{L}_V^n$ into the vector search structure $S_{n, |V|}$.
    \item Now, suppose you are given a target tuple $t_A$, that is associated with a set $A$ of lineage vectors of cardinality $|A| \in [1, M]$. Construct $|A| \times k$ long target vectors $\vec{\tau}_{1, 1}^k, ..., \vec{\tau}_{|A|, k}^k$, for each $k \in [1, M]$.
    \item Hereafter, we denote a set $V$ of lineage vectors with cardinality $k$ as $V^k$.
    \item For each $k \in [1, M]$, we look \textit{separately} for the closest (dot-product wise) candidate long vector $\vec{L}_{V_{i, j}^k}^{n=|A|} \in \mathbb{R}^{|A| \times k \times D}$ (and its respective candidate tuple $t_{V_{i, j}^k}$) in $S_{|A|, k}$, to each $\vec{\tau}_{i, j}^k \in \mathbb{R}^{|A| \times k \times D}$, respectively. 
    Intuitively, this focuses on candidate tuples associated with sets of vectors of cardinality $k$.
    \item 
    Next, intuitively, we need to choose the ``best" one among the ``winners" of different $k$ values.
    We compute the similarity scores $\vec{\tau}_{1, 1}^k \cdot \vec{L}_{V_{1, 1}^k}^{|A|}, ..., \vec{\tau}_{|A|, 1}^k \cdot \vec{L}_{V_{|A|, 1}^k}^{|A|}, ..., \vec{\tau}_{1, k}^k \cdot \vec{L}_{V_{1, k}^k}^{|A|}, ..., \vec{\tau}_{|A|, k}^k \cdot \vec{L}_{V_{|A|, k}^k}^{|A|}$, for each $k \in [1, M]$ (a total of $\sum_{k=1}^M |A| \times k = |A| \times \sum_{k=1}^M k = |A| \times \frac{M(1 + M)}{2}$ computations). The one yielding the highest score, say $\vec{L}_{V_{{\Tilde{i}, {\Tilde{j}}}}^{\Tilde{k}}}^{|A|}$, identifies the desired candidate tuple $t_{V_{{\Tilde{i}, {\Tilde{j}}}}^{\Tilde{k}}}$, which is associated with the set $V_{{\Tilde{i}, {\Tilde{j}}}}^{\Tilde{k}}$ of lineage vectors, according to our set-oriented similarity formula.
\end{enumerate}
