# Supplementary material for: ML Based Lineage in Databases
Source: arXiv:2109.06339 source file (2021-10-03)
Supplement: Supplementary file 4 [file appendix_movielens_schema.tex]

\chapter{MovieLens Dataset}
\label{appendix:movielens_schema}

Following is a detailed description of the data fields, of each table in the MovieLens dataset (used in the experiments in chapter \ref{chap:experimental_evaluation}).

\section{\texttt{movies}}\label{appendix:sec:movies}
\begin{itemize}
    \item \textbf{\texttt{movieId}} - a number that uniquely identifies a movie item. Links to the \texttt{ratings} table and the \texttt{tags} table. These movie ids are consistent with those used on the MovieLens web site (e.g., id 1 corresponds to the URL \url{https://movielens.org/movies/1}).
    \item \textbf{\texttt{title}} - movie titles, which are entered manually or imported from \url{https://www.themoviedb.org/}, and include the year of release in parentheses.
    \item \textbf{\texttt{genres}} - genres are a pipe-separated list, and are selected from the following:
    \begin{itemize}
        \item Action
        \item Adventure
        \item Animation
        \item Children's
        \item Comedy
        \item Crime
        \item Documentary
        \item Drama
        \item Fantasy
        \item Film-Noir
        \item Horror
        \item Musical
        \item Mystery
        \item Romance
        \item Sci-Fi
        \item Thriller
        \item War
        \item Western
        \item (no genres listed)
    \end{itemize}
\end{itemize}

\section{\texttt{ratings}}\label{appendix:sec:ratings}
% \subsection{Fields Description}
\begin{itemize}
    \item \textbf{\texttt{userId}} - a number that uniquely identifies a user. Links to the \texttt{tags} table.
    \item \textbf{\texttt{movieId}} - a number that uniquely identifies a movie item. Links to the \texttt{movies} table and the \texttt{tags} table. These movie ids are consistent with those used on the MovieLens web site (e.g., id 1 corresponds to the URL \url{https://movielens.org/movies/1}).
    \item \textbf{\texttt{rating}} - a rating of the movie identified by \texttt{movieId}, rated by the user identified by \texttt{userId}. Ratings are made on a 5-star scale, with half-star increments (0.5 stars - 5.0 stars).
    \item \textbf{\texttt{timestamp}} - a timestamp of the rating action. Timestamps represent seconds since midnight Coordinated Universal Time (UTC) of January 1, 1970.
\end{itemize}
% \subsection{Sample}
% \input{tables/bfpdb_samples/nutrients}

\section{\texttt{tags}}\label{appendix:sec:tags}
\begin{itemize}
    \item \textbf{\texttt{userId}} - a number that uniquely identifies a user. Links to the \texttt{ratings} table.
    \item \textbf{\texttt{movieId}} - a number that uniquely identifies a movie item. Links to the \texttt{movies} table and the \texttt{ratings} table. These movie ids are consistent with those used on the MovieLens web site (e.g., id 1 corresponds to the URL \url{https://movielens.org/movies/1}).
    \item \textbf{\texttt{tag}} - tags are user-generated metadata about movies. Each tag is typically a single word or short phrase. The meaning, value, and purpose of a particular tag is determined by each user.
    \item \textbf{\texttt{timestamp}} - a timestamp of the tagging action. Timestamps represent seconds since midnight Coordinated Universal Time (UTC) of January 1, 1970.
\end{itemize}
