# Supplementary material for: ML Based Lineage in Databases
Source: arXiv:2109.06339 source file (2021-10-03)
Supplement: Supplementary file 5 [file appendix_training_word_vectors.tex]

\section{Training Word Vectors}
\label{appendix:training-word-vectors}

\par We solve these problems by properly setting hyperparameters (e.g., window size), artificially (and carefully) injecting repeated text inside a sentence, and dividing the training into multiple, different stages. 
A detailed outline of the ``textification'' and training processes follows:
\begin{enumerate*}
    \item Generate a \texttt{Key} column with unique values for each table in the DB.
    \item Extract two corpora from the DB, one with columns (except the \texttt{Key} columns) as sentences, and the other with tuples as sentences.
    \item Transform each numerical value in the generated corpora by concatenating the relevant column name to the number. Other methods of dealing with numerical values exist as well, and are discussed in section \ref{sec:relational_embedding}.
    \item Transform each sentence in the generated corpora by injecting the corresponding \texttt{Key} value repeatedly after every $k$ (a separate hyperparameter for the columns corpus and the tuples corpus) words in the sentence. The idea is to encode more information about each tuple in its corresponding \texttt{Key} value vector.
    \item Incrementally train a \textsc{Word2Vec} model on the generated corpora. First, train on the columns corpus and then on the tuples corpus. One may question why we have the same model for both the tuple-based (see section \ref{chap:per_tuple_lineage_vectors}) and the column-based (see section \ref{chap:per_column_lineage_vectors}) lineage vectors. The answer is that experimentally the models that are restricted to only the tuples corpus or only the columns corpus yield inferior results.
\end{enumerate*}
One more interesting caveat, of dealing with texts extracted from relations, is that missing data (empty/null cells) is sometimes automatically converted (when an external tool, e.g., Python, is used to interface with PostgreSQL) to `None'. Given that `None' is not a \textit{stop word} (words that are removed from a corpus as part of a common practice of cleanup before training), we realized that `None' adds noise to the vectors (if there is a lot of missing data in the DB). Adding `None' to the list of \textsc{Word2Vec} stop words improved drastically both the word embedding model quality and the overall accuracy of our system.
