# Supplementary material for: ML Based Lineage in Databases
Source: arXiv:2109.06339 source file (2021-10-03)
Supplement: Supplementary file 7 [file exp1.tex]

% \begin{adjustbox}{width=\columnwidth,center}
\begin{figure}[H]
% \raggedright
% \begin{small}
    \texttt{
    % \textcolor{white}{\tiny something}\\
    \textcolor{white}{F}\sqlcolor{SELECT} prt.\fieldcolor{manufacturer} \\
    \textcolor{white}{FF}\sqlcolor{FROM} protein prt, (\sqlcolor{SELECT DISTINCT} \fieldcolor{manufacturer} \sqlcolor{FROM} prepared) t\\
    \textcolor{white}{FF}\sqlcolor{WHERE POSITION}(\strcolor{'sugar'} \sqlcolor{IN} prt.\fieldcolor{ingredients}) > \numcolor{0} \\
    \textcolor{white}{FF}\sqlcolor{AND} prt.\fieldcolor{manufacturer} = t.\fieldcolor{manufacturer}\\
    \textcolor{white}{FF}\sqlcolor{GROUP BY} prt.\fieldcolor{manufacturer}
    }
    % \textbf{\caption{\label{fig:queries_usda_bpfd}Running example query for the USDA Branded Products Food Database}}
% \end{small}
\end{figure}
% \end{adjustbox}
