# Supplementary material for: ML Based Lineage in Databases
Source: arXiv:2109.06339 source file (2021-10-03)
Supplement: Supplementary file 10 [file exp4.tex]

% \begin{adjustbox}{width=\columnwidth,center}
\begin{figure}[H]
% \raggedright
% \begin{small}
    \texttt{
    % \textcolor{white}{\tiny something}\\
    \textcolor{white}{F}\sqlcolor{SELECT} n.\fieldcolor{ndb\_no}, n.\fieldcolor{derivation\_code} \\
    \textcolor{white}{FF}\sqlcolor{FROM} $\texttt{exp}\sb\texttt{1}$, $\texttt{exp}\sb\texttt{2}$, products p, nutrients n\\
    \textcolor{white}{FF}\sqlcolor{WHERE} ($\texttt{exp}\sb\texttt{1}$.\fieldcolor{manufacturer} = p.\fieldcolor{manufacturer}\\
    \textcolor{white}{FFFFFF}\sqlcolor{OR} $\texttt{exp}\sb\texttt{2}$.\fieldcolor{manufacturer} = p.\fieldcolor{manufacturer}) \\
    \textcolor{white}{FF}\sqlcolor{AND} p.\fieldcolor{ndb\_no} = n.\fieldcolor{ndb\_no}\\
    \textcolor{white}{FF}\sqlcolor{GROUP BY} n.\fieldcolor{ndb\_no}, n.\fieldcolor{derivation\_code} \sqlcolor{LIMIT} \numcolor{10}
    }
    % \textbf{\caption{\label{fig:queries_usda_bpfd}Running example query for the USDA Branded Products Food Database}}
% \end{small}
\end{figure}
% \end{adjustbox}
