# Supplementary material for: ML Based Lineage in Databases
Source: arXiv:2109.06339 source file (2021-10-03)
Supplement: Supplementary file 11 [file exp5.tex]

% \begin{adjustbox}{width=\columnwidth,center}
\begin{figure}[H]
% \raggedright
% \begin{small}
    \texttt{
    % \textcolor{white}{\tiny something}\\
    \textcolor{white}{F}\sqlcolor{SELECT DISTINCT} rtd.\fieldcolor{name} \\
    \textcolor{white}{FF}\sqlcolor{FROM} $\texttt{exp}\sb\texttt{2}$, readytodrink rtd\\
    \textcolor{white}{FF}\sqlcolor{WHERE} $\texttt{exp}\sb\texttt{2}$.\fieldcolor{manufacturer} = rtd.\fieldcolor{manufacturer}\\
    \textcolor{white}{FF}\sqlcolor{AND POSITION}(\strcolor{'mango'} \sqlcolor{IN} rtd.\fieldcolor{name}) > \numcolor{0}
    }
    % \textbf{\caption{\label{fig:queries_usda_bpfd}Running example query for the USDA Branded Products Food Database}}
% \end{small}
\end{figure}
% \end{adjustbox}
