# Supplementary material for: ML Based Lineage in Databases
Source: arXiv:2109.06339 source file (2021-10-03)
Supplement: Supplementary file 12 [file prepared.tex]

\newcommand{\sqlcolor}[1]{\textcolor{Bittersweet}{#1}}
\newcommand{\fieldcolor}[1]{\textcolor{Fuchsia}{#1}}
\newcommand{\strcolor}[1]{\textcolor{ForestGreen}{#1}}

% \begin{adjustbox}{width=\columnwidth,center}
\begin{figure}[h]
% \raggedright
% \begin{small}
    \texttt{
    % \textcolor{white}{\tiny something}\\
    \textcolor{white}{F}\sqlcolor{SELECT} p.\fieldcolor{ndb\_no}, p.\fieldcolor{manufacturer}, p.\fieldcolor{name}, p.\fieldcolor{ingredients} \\
    \textcolor{white}{FF}\sqlcolor{FROM} products p, serving\_size ss\\
    \textcolor{white}{FF}\sqlcolor{WHERE} p.\fieldcolor{ndb\_no} = ss.\fieldcolor{ndb\_no} \\ 
    \textcolor{white}{FF}\sqlcolor{AND} ss.\fieldcolor{preparation\_state} = \strcolor{'prepared'}
    }
    % \textbf{\caption{\label{fig:queries_usda_bpfd}Running example query for the USDA Branded Products Food Database}}
% \end{small}
\end{figure}
% \end{adjustbox}
